# Supplementary material for: Mesh Neural Networks for SE(3)-Equivariant Hemodynamics Estimation on the Artery Wall
Source: arXiv:2212.05023 source file (2024-06-14)
Supplement: Supplementary file 1 [file experiments.tex]

\section{}\label{app:wallclock}

\begin{table}[h]
	\begin{center}
    	\caption{\textbf{Training time until convergence} measured in number of epochs and wall-clock time of parallelised training on two NVIDIA A40 GPUs.}
    	
    	\begin{tabular}{@{}cccccc@{}}
    		\toprule
    		& \multicolumn{2}{c}{\# epochs} && \multicolumn{2}{c}{Wall-clock time [h]}\\
    		\cmidrule{2-3} \cmidrule{5-6}
    		& single & bifurcating && single & bifurcating\\
    		\midrule
    		IsoGCN & 1145 & \phantom{0}270 && 10:03 & \phantom{0}6:13\\
    		AttGCN & 1470 & \phantom{0}660 && 31:18 & 30:48\\
    		PointNet\texttt{++} & 3920 & 1600 && 20:48 & 35:01\\
    		\midrule
    		GEM-GCN & \phantom{0}700 & \phantom{0}165 && 22:24 & 15:57\\
    		PointNet\texttt{++}$^\ddagger$ & 6735 & 3330 && 31:29 & 57:16\\
    		\bottomrule
    		\multicolumn{6}{l}{$^\ddagger$ trained under data augmentation (random rotation in 3D)}
    	\end{tabular}
    	\label{tab:wallclock}
	\end{center}
\end{table}

Table~\ref{tab:wallclock} lists the number of epochs and the wall-clock time required for convergence, indicated by a plateau in training and validation loss, of GEM-GCN and PointNet++ on the full training set. We find that  GEM-GCN converges in considerably fewer epochs than PointNet\texttt{++}. In terms of wall-clock time, GEM-GCN takes slightly longer than PointNet\texttt{++} and considerably more time than IsoGCN for the single arteries, while AttGCN takes the most time. GEM-GCN has the highest ratio of wall-clock time to epochs because its message passing contains high-order tensor products (details in \cite{HaanWeiler2021}) which require a lot of computational work. However, the included group symmetry acts as loss regularisation that accelerates the convergence in terms of epochs. We find that PointNet\text{++} and AttGCN are disproportionally harder to train on the bifurcating artery dataset compared to GEM-GCN and IsoGCN. We have no proper explanation for this but hint at the fact that both PointNet\text{++} and AttGCN work with neighbourhood attention scaling which seems to harmonise better with the single artery dataset.

\section{}

\begin{figure}[h]
    \centering
    \includegraphics[width=\columnwidth]{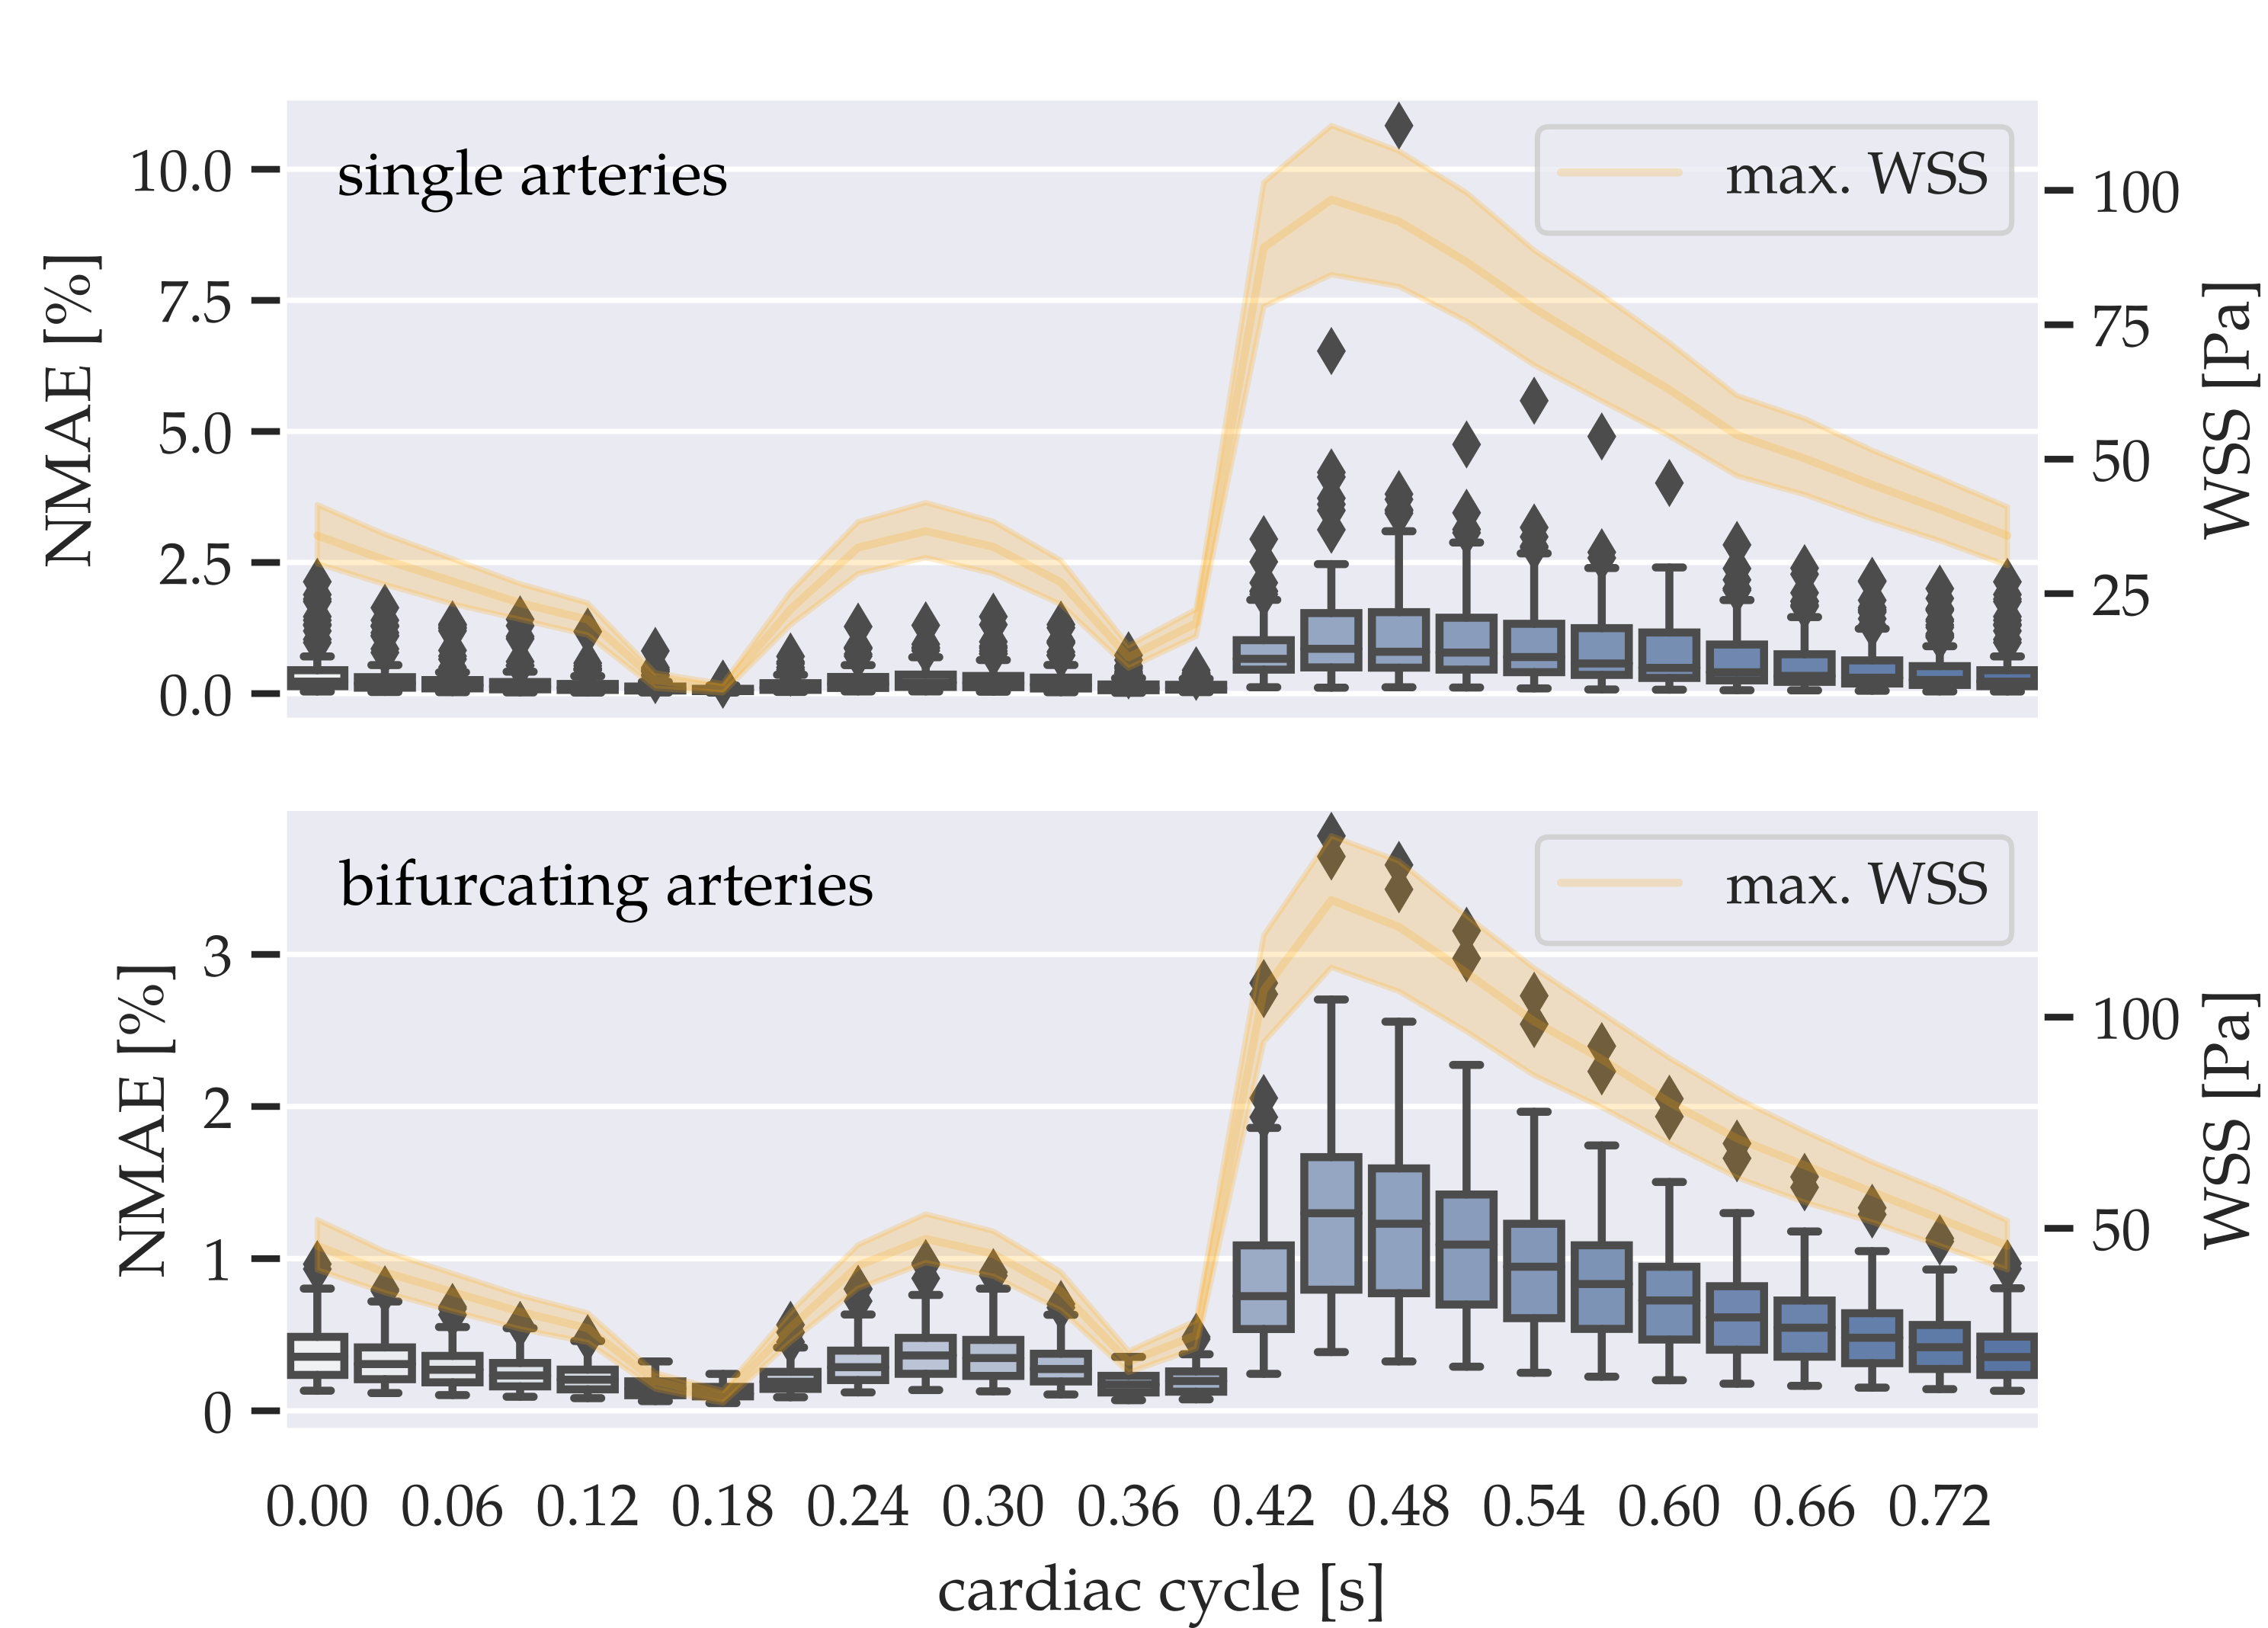}
    \caption{\textbf{Conditional, pulsatile} single (top) and bifurcating (bottom) artery WSS prediction error across the test split over time. Five boundary conditions per artery are contained as separate data points. Maximum WSS magnitude is indicated in yellow.}
    \label{plt:bct}
\end{figure}
\begin{figure}[ht]
    \centering
    \includegraphics[width=\columnwidth]{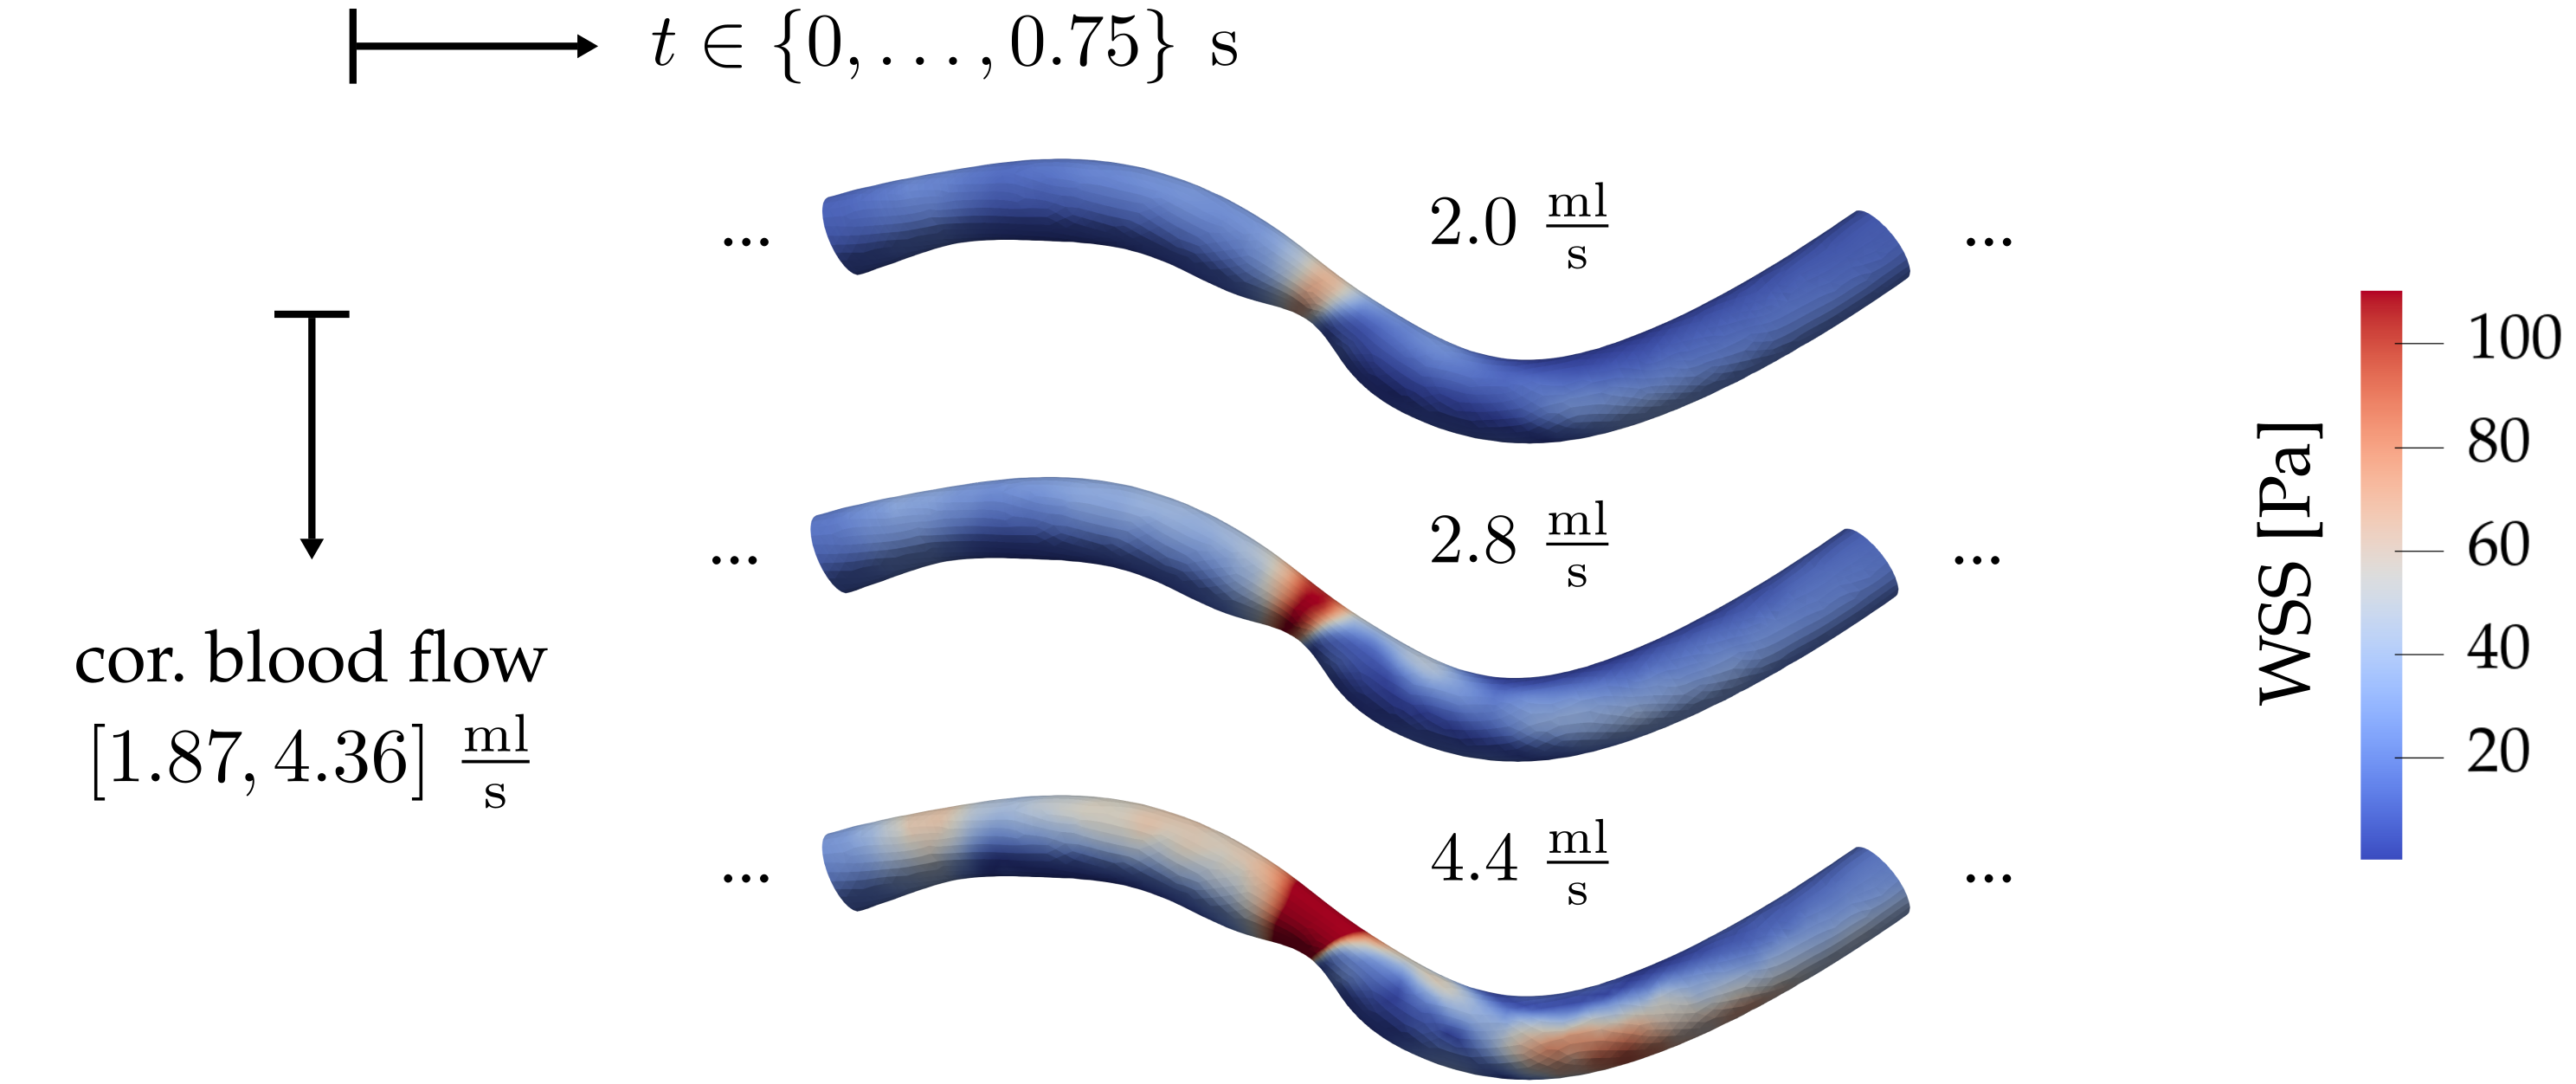}
    \caption{\textbf{Conditional, pulsatile} single-artery WSS prediction. GEM-GCN is conditioned on coronary blood flow and maps boundary conditions to according wall shear stress.}
    \label{fig:bct}
\end{figure}
